# Supplementary material for: Quantum Circuits for Sparse Isometries
Source: arXiv:2006.00016 ancillary file (2021-03-09)
Supplement: Supplementary file 1 [file supplementary_data.pdf]

# Data for Fig. 4

Emanuel Malvetti,[1,*] Raban Iten,[2,†] and Roger Colbeck[3,‡]
[1]Department of Chemistry, TUM, Lichtenbergstraße 4, 85747 Garching, Germany
[2]ETH Zürich, 8093 Zürich, Switzerland
[3]Department of Mathematics, University of York, YO10 5DD, UK
(Dated: 2nd December 2020)

| $s = 1$ | | | | | | | | | | | | | | | |
|---|---|---|---|---|---|---|---|---|---|---|---|---|---|---|---|
| $n = 3$ | | $n = 4$ | | $n = 5$ | | $n = 6$ | | $n = 7$ | | $n = 8$ | | $n = 9$ | | $n = 10$ | |
| C-NOTs | # | C-NOTs | # | C-NOTs | # | C-NOTs | # | C-NOTs | # | C-NOTs | # | C-NOTs | # | C-NOTs | # |
| 0 | 99 | 0 | 46 | 0 | 35 | 0 | 24 | 0 | 10 | 0 | 7 | 0 | 7 | 0 | 1 |
| 1 | 46 | 1 | 42 | 1 | 21 | 1 | 16 | 1 | 8 | 1 | 4 | 1 | 4 | 1 | 2 |
| 2 | 35 | 2 | 47 | 2 | 34 | 2 | 34 | 2 | 20 | 2 | 14 | 2 | 6 | 2 | 7 |
| 3 | 20 | 3 | 45 | 3 | 64 | 3 | 62 | 3 | 60 | 3 | 48 | 3 | 35 | 3 | 21 |
| | | 4 | 20 | 4 | 40 | 4 | 47 | 4 | 59 | 4 | 53 | 4 | 44 | 4 | 44 |
| | | | | 5 | 6 | 5 | 16 | 5 | 30 | 5 | 48 | 5 | 47 | 5 | 52 |
| | | | | | | 6 | 1 | 6 | 9 | 6 | 20 | 6 | 37 | 6 | 33 |
| | | | | | | | | 7 | 4 | 7 | 4 | 7 | 19 | 7 | 23 |
| | | | | | | | | | | 8 | 2 | 8 | 1 | 8 | 12 |
| | | | | | | | | | | | | | | 9 | 5 |

*Electronic address: emanuel.malvetti@tum.de
†Electronic address: itenr@itp.phys.ethz.ch
‡Electronic address: roger.colbeck@york.ac.uk

| $s = 2$ | | | | | | | | | | | | | |
|---|---|---|---|---|---|---|---|---|---|---|---|---|---|
| $n = 4$ | | $n = 5$ | | $n = 6$ | | $n = 7$ | | $n = 8$ | | $n = 9$ | | $n = 10$ | |
| C-NOTs | # | C-NOTs | # | C-NOTs | # | C-NOTs | # | C-NOTs | # | C-NOTs | # | C-NOTs | # |
| 1 | 3 | 1 | 1 | 4 | 2 | 5 | 1 | 6 | 1 | 9 | 1 | 9 | 2 |
| 4 | 29 | 4 | 3 | 5 | 2 | 7 | 2 | 8 | 1 | 10 | 4 | 10 | 1 |
| 5 | 35 | 5 | 16 | 6 | 2 | 8 | 2 | 10 | 6 | 11 | 2 | 11 | 2 |
| 6 | 22 | 6 | 14 | 7 | 6 | 9 | 6 | 11 | 15 | 12 | 19 | 12 | 7 |
| 7 | 23 | 7 | 13 | 8 | 16 | 10 | 25 | 12 | 30 | 13 | 16 | 13 | 13 |
| 8 | 33 | 8 | 20 | 9 | 27 | 11 | 34 | 13 | 33 | 14 | 22 | 14 | 9 |
| 9 | 40 | 9 | 48 | 10 | 46 | 12 | 32 | 14 | 22 | 15 | 18 | 15 | 18 |
| 10 | 15 | 10 | 46 | 11 | 46 | 13 | 42 | 15 | 5 | 16 | 6 | 16 | 8 |
| | | 11 | 28 | 12 | 29 | 14 | 23 | 16 | 13 | 17 | 19 | 17 | 8 |
| | | 12 | 10 | 13 | 13 | 15 | 7 | 17 | 21 | 18 | 20 | 18 | 21 |
| | | 13 | 1 | 14 | 3 | 16 | 12 | 18 | 19 | 19 | 25 | 19 | 24 |
| | | | | 15 | 4 | 17 | 10 | 19 | 17 | 20 | 17 | 20 | 28 |
| | | | | 16 | 4 | 18 | 2 | 20 | 13 | 21 | 16 | 21 | 30 |
| | | | | | | 19 | 1 | 21 | 4 | 22 | 14 | 22 | 14 |
| | | | | | | 20 | 1 | | | 25 | 1 | 23 | 11 |
| | | | | | | | | | | | | 24 | 3 |
| | | | | | | | | | | | | 26 | 1 |

| $s=3$ | | | | | | | | | | $s=4$ | | | | | |
|---|---|---|---|---|---|---|---|---|---|---|---|---|---|---|---|
| $n=6$ | | $n=7$ | | $n=8$ | | $n=9$ | | $n=10$ | | $n=8$ | | $n=9$ | | $n=10$ | |
| C-NOTs | # | C-NOTs | # | C-NOTs | # | C-NOTs | # | C-NOTs | # | C-NOTs | # | C-NOTs | # | C-NOTs | # |
| 35 | 3 | 37 | 1 | 51 | 1 | 60 | 2 | 63 | 1 | 199 | 1 | 206 | 1 | 228 | 1 |
| 36 | 1 | 39 | 1 | 53 | 3 | 61 | 2 | 64 | 1 | 200 | 3 | 219 | 1 | 244 | 1 |
| 37 | 1 | 47 | 2 | 56 | 1 | 62 | 2 | 65 | 4 | 201 | 3 | 220 | 1 | 245 | 2 |
| 38 | 1 | 48 | 7 | 59 | 3 | 63 | 7 | 66 | 2 | 202 | 3 | 221 | 1 | 246 | 5 |
| 39 | 3 | 49 | 4 | 60 | 7 | 64 | 8 | 67 | 6 | 203 | 4 | 222 | 3 | 247 | 7 |
| 40 | 1 | 50 | 5 | 61 | 14 | 65 | 10 | 68 | 1 | 206 | 1 | 224 | 4 | 248 | 3 |
| 44 | 2 | 51 | 7 | 62 | 22 | 66 | 8 | 69 | 4 | 215 | 1 | 226 | 2 | 249 | 5 |
| 45 | 1 | 52 | 4 | 63 | 13 | 67 | 2 | 73 | 3 | 216 | 5 | 227 | 2 | 250 | 2 |
| 46 | 12 | 53 | 1 | 64 | 21 | 69 | 2 | 74 | 2 | 217 | 10 | 228 | 1 | 254 | 2 |
| 47 | 15 | 57 | 1 | 65 | 13 | 70 | 2 | 75 | 9 | 218 | 13 | 234 | 1 | 259 | 1 |
| 48 | 20 | 58 | 14 | 66 | 10 | 71 | 1 | 76 | 13 | 219 | 11 | 237 | 2 | 260 | 1 |
| 49 | 19 | 59 | 15 | 68 | 2 | 72 | 3 | 77 | 15 | 220 | 9 | 239 | 8 | 262 | 4 |
| 50 | 10 | 60 | 30 | 70 | 3 | 73 | 8 | 78 | 21 | 221 | 13 | 240 | 6 | 263 | 12 |
| 51 | 3 | 61 | 35 | 71 | 4 | 74 | 15 | 79 | 24 | 222 | 9 | 241 | 17 | 264 | 13 |
| 52 | 1 | 62 | 24 | 72 | 15 | 75 | 25 | 80 | 35 | 223 | 5 | 242 | 13 | 265 | 11 |
| 55 | 1 | 63 | 17 | 73 | 15 | 76 | 32 | 81 | 24 | 224 | 5 | 243 | 11 | 266 | 18 |
| 56 | 6 | 64 | 3 | 74 | 16 | 77 | 16 | 82 | 10 | 225 | 2 | 244 | 20 | 267 | 22 |
| 57 | 15 | 65 | 4 | 75 | 17 | 78 | 31 | 83 | 13 | 226 | 2 | 245 | 10 | 268 | 20 |
| 58 | 30 | 66 | 1 | 76 | 12 | 79 | 10 | 84 | 6 | 227 | 1 | 246 | 8 | 269 | 15 |
| 59 | 23 | 68 | 1 | 77 | 5 | 80 | 8 | 85 | 2 | 231 | 1 | 247 | 8 | 270 | 19 |
| 60 | 22 | 69 | 7 | 78 | 3 | 81 | 5 | 89 | 1 | 233 | 1 | 248 | 2 | 271 | 14 |
| 61 | 5 | 70 | 5 | | | 88 | 1 | 90 | 1 | 234 | 3 | 249 | 2 | 272 | 4 |
| 62 | 4 | 71 | 2 | | | | | 93 | 1 | 235 | 1 | 252 | 1 | 273 | 1 |
| 63 | 1 | 72 | 7 | | | | | 94 | 1 | 236 | 9 | 257 | 1 | 274 | 4 |
| | | 73 | 1 | | | | | | | 237 | 13 | 258 | 3 | 275 | 1 |
| | | 76 | 1 | | | | | | | 238 | 12 | 259 | 3 | 280 | 1 |
| | | | | | | | | | | 239 | 14 | 260 | 11 | 285 | 1 |
| | | | | | | | | | | 240 | 15 | 261 | 8 | 287 | 6 |
| | | | | | | | | | | 241 | 16 | 262 | 12 | 288 | 3 |
| | | | | | | | | | | 242 | 6 | 263 | 11 | 289 | 1 |
| | | | | | | | | | | 243 | 2 | 264 | 7 | | |
| | | | | | | | | | | 244 | 3 | 265 | 8 | | |
| | | | | | | | | | | 254 | 1 | 266 | 6 | | |
| | | | | | | | | | | 259 | 1 | 267 | 3 | | |
| | | | | | | | | | | 260 | 1 | 268 | 2 | | |
